# Supplementary material for: The Protein Force Field Plays a Crucial Role in Obtaining Accurate Macromolecular Ensembles of IDPs
Source: arXiv:2508.18570 source file (2025-08-26)
Supplement: Supplementary file 1 [file suppl.pdf]

# Supporting Information For

# The Protein Force Field Plays a Crucial Role in Obtaining Accurate Macromolecular Ensembles of IDPs

Rohan S. Adhikari,[*,†,‡] Winnie H. Shi,[†] Amanda B. Marciel,[*,†] and Walter G. Chapman[*,†]

†*Department of Chemical and Biomolecular Engineering, Rice University, 6100 Main St., Houston, TX 77005, USA*

‡*Department of Chemical and Biomolecular Engineering, University of Delaware, Newark, DE 19716, USA*

E-mail: rohana@udel.edu; am152@rice.edu; wgchap@rice.edu

# S.1 Additional Simulation Details

Linear chains of the three polyampholyte sequences [$(EK)_{16}$, $(E_2K_2)_8$, and $(E_4K_4)_4$] are built using the PeptideBuilder package.[1] The linear EK polyampholytes are simulated using the generalized Born surface/accessible (GB/SA) implicit solvent model[2] on the NAMD program[3] for 100 ns. The most probable polyampholyte conformation in the last 50 ns of the GB/SA simulation are determined by binning the radius of gyration and end-to-end distance metrics. The most probable polyampholyte conformations from the GB/SA simulations are used as the starting structure for the explicit water MD simulations.

The three polyampholyte sequences are simulated with three different force field combinations. The AMBER ff99SB atomistic force field for proteins is paired with the TIP3P water model to obtain the first combination (TFF99). The AMBER ff99SB protein force field is paired with the OPC waters for the second combination (OFF99). The AMBER ff19SB protein force field is paired with the OPC waters to obtain the third combination (FF19O). The three polyampholyte sequences are studied with the three force field combinations for a total of nine simulation systems. The topology files for the nine simulation systems are obtained using the AMBERTools package.[4] The mass of the solute hydrogens are changed to 3.024 a.u. using hydrogen mass repartitioning (HMR). In HMR, the mass of the parent solute atom (bonded to hydrogen) is reduced to maintain a constant solute mass.[5] HMR allows the time step of the simulation to be increased to 4 fs.

The TFF99 simulation boxes are packed with one EK polyampholyte and 29800 TIP3P waters using the PACKMOL package.[6] The OFF99 and FF19O simulation boxes are packed with one EK polyampholyte and 57600 OPC waters using PACKMOL. All nine simulation systems are energy minimized using the conjugate-gradient energy minimization for 2000 cycles by using a restraint of 5 kcal/mol/Å$^2$ on the solute atoms. The restraints on the solute atoms are removed in three stages by reducing the restraint values successively to 5, 0.5, 0.05 kcal/mol/Å$^2$ and simulating the systems using a 1 fs time step for $1*10^6$ time steps each. After this step, the restraints on the solute are removed and the simulations are run at 293.15 K and 1 atm pressure using a 4 fs time step. All nine simulations are run for a total of 8 $\mu$s each using the AMBER20 simulation package.[7] The

simulation frames are saved to the trajectory file once every 40 ps ($1*10^4$ time steps) during the last 4 $\mu$s of the simulation (production phase).

Bulk water simulations of the TIP3P and OPC waters are performed using a 4 fs time step. 29800 TIP3P waters are simulated at 293.15 K and 1 atm pressure which gives a cubic box of size $\approx$ 96*96*96 Å, 57600 OPC waters are simulated at 293.15 K and 1 atm pressure which gives a cubic box of size $\approx$ 120*120*120 Å. 5000 simulation frames in the last 40 ns of the simulation are saved for each of the TIP3P and OPC water simulations.

A Langevin thermostat with a collision frequency ($\gamma_{ln}$) of 1 ps$^{-1}$ is used to maintain the temperature at 293.15 K for all the simulations performed. A Monte Carlo barostat with a pressure relaxation time ($\tau_\text{p}$) of 1.0 ps is used to maintain the pressure at 1 atm for all the simulations performed.

## S.2 Additional Details of the Scattering Computation

The scattering profiles from the simulations are computed using a simulated background subtraction procedure which is represented in Eq. S.1.

$$\Delta I(q) = I_{\mathrm{A}}(q) - I_{\mathrm{B}}(q) \tag{S.1}$$

For explicit water MD simulations, Park et al.[8] developed a framework that translates Eq. S.1 to a form that accounts for the hydration layer waters in atomic detail (shown in Eq. S.2).

$$\Delta I(q) = \left\langle \left|\langle A(\mathbf{q})\rangle' - \langle B(\mathbf{q})\rangle''\right|^2 + \left[\langle |A(\mathbf{q})|^2\rangle' - \left|\langle A(\mathbf{q})\rangle'\right|^2\right] - \left[\langle |B(\mathbf{q})|^2\rangle'' - \left|\langle B(\mathbf{q})\rangle''\right|^2\right] \right\rangle_{\Omega} \tag{S.2}$$

$A(\mathbf{q})$ is the amplitude calculated from the protein-water simulation. $B(\mathbf{q})$ is the amplitude calculated from the bulk-water simulation. In Eq. S.2, $\langle ... \rangle'$, $\langle ... \rangle''$, and $\langle ... \rangle_{\Omega}$ denote the ensemble average over the simulation frames in the biomolecule in solvent simulation, ensemble average over the simulation frames in the bulk solvent simulation, and an orientational average of the scattering intensities. The orientational average shown in Eq. S.2 is performed using 1500 orientational vectors with the method of spirals.[9] The computation for $A(\mathbf{q})$ and $B(\mathbf{q})$ are shown in Eq. S.3. Where the summations run over all atoms in the envelope of the protein-water simulation ($N_A$) and all atoms in the envelope of the bulk-water simulation ($N_B$) respectively. The form factors ($f_j$) for the atoms are obtained from International Tables for Crystallography Vol. C.[10] The form factors of the oxygens and hydrogens of the water molecule are corrected to account for the polarizability of water using Sorenson's correction.[11]

$$A(\mathbf{q}) = \sum_{j=1}^{N_A} f_j(q) e^{-i\mathbf{q}.r_j},$$
$$B(\mathbf{q}) = \sum_{j=1}^{N_B} f_j(q) e^{-i\mathbf{q}.r_j} \tag{S.3}$$

The envelope for the scattering computation should include regions where the density of the waters are different compared to the bulk density of the waters. For polypeptides in water, moving a distance of 7 Å away from all the solute atoms is found to be enough to obtain bulk-like behavior of waters. For frozen protein atoms as considered by Park et al.,[8] defining an envelope that encapsulates all density variations in the water is relatively simple. Chen and Hub[12] showed how to define an envelope that encapsulates all the solvent density variation around a thermally fluctuating solute by defining an icosphere whose vertices are moved 7 Å away from all the solute atoms of all simulation frames. In the SWAXS-AMDE package, the envelope is defined by radiating 20594 direction vectors from the center of mass of the thermally fluctuating protein and moving the direction vectors 7 Å away from all solute atoms of all simulation frames. A water molecule is considered for the scattering computation if it is determined to be inside this envelope defined by the 20594 direction vectors.

Solvent density corrections are applied to the scattering amplitudes [$A(\mathbf{q})$ and $B(\mathbf{q})$] to account for the bulk density variations due to the finite size of the simulation box and the finite number of simulation frames following the procedure reported in Ref. 12.

The $I(q)$s are computed at 139 $q$ values in the range of [0.017-0.5] Å$^{-1}$ for a comparison against experiments. The error bars in the experimental $I(q)$ in the range of [0.007-0.017) Å$^{-1}$ are as high as 20 %, hence the $q$-range for comparison between experiments and simulations is restricted to [0.017-0.5] Å$^{-1}$. The scattering intensities for each of the nine simulation systems are computed from five blocks of 1000 simulation frames. The mean and error bars of the scattering intensities [I(q)] from the five blocks are reported in this study for the nine simulation systems.

## S.3 Validation of SWAXS-AMDE

To validate the SWAXS-AMDE model, we reproduce the scattering calculation reported by Chen and Hub[12] for lysozyme (PDB code: 193L). Lysozyme is packed in a simulation box with 33054 water molecules and 8 chloride ions (counter ions). The MD simulation of lysozyme in water is performed on GROMACS[13] with the CHARMM27 force field for the protein and TIP3P waters. The temperature is set to 300 K and the pressure is set to 1 bar. All bonds involving hydrogens are constrained using LINCS. The Lennard Jones (LJ) dispersion interactions are cut off at 10 Å (with long-range dispersion corrections for energy and pressure) and the PME grid spacing is set to 1.2 Å. 100 ps of NVT equilibration is performed after minimization followed by a 100 ps of NPT equilibration by applying position restraints to the backbone atoms of lysozyme (k = 1000 kJ $mol^{-1}$ $nm^{-2}$). The box size of the simulation is around 101*101*101 Å. After equilibration, we perform 10 ns of NPT production phase MD simulation (with a 2 fs time step) and save the protein-solvent trajectories once every 10 ps. Similar procedure is repeated to collect the trajectory of bulk TIP3P waters.

The protein-solvent and bulk-solvent trajectories are analyzed using SWAXS-AMDE for a 101 $q$ values between 0.0 to 1.0 $Å^{-1}$. An envelope is defined for the scattering calculation such that it is at least 8 Å away from all solute atoms from all simulation frames. Solvent density corrections are applied to the scattering calculations by fixing the bulk density of water to 0.334 e/$Å^3$. The 1000 simulation frames are grouped into blocks of 200 (5 blocks) and the SWAXS-AMDE scattering calculation is performed for the five blocks to report error bars. The SWAXS-AMDE computed scattering profiles (with error bars) for lysozyme (PDB code: 193L) are reported in Fig. S1 and are in excellent quantitative agreement with the results reported by Chen and Hub [Figure 5B in Ref. 12].

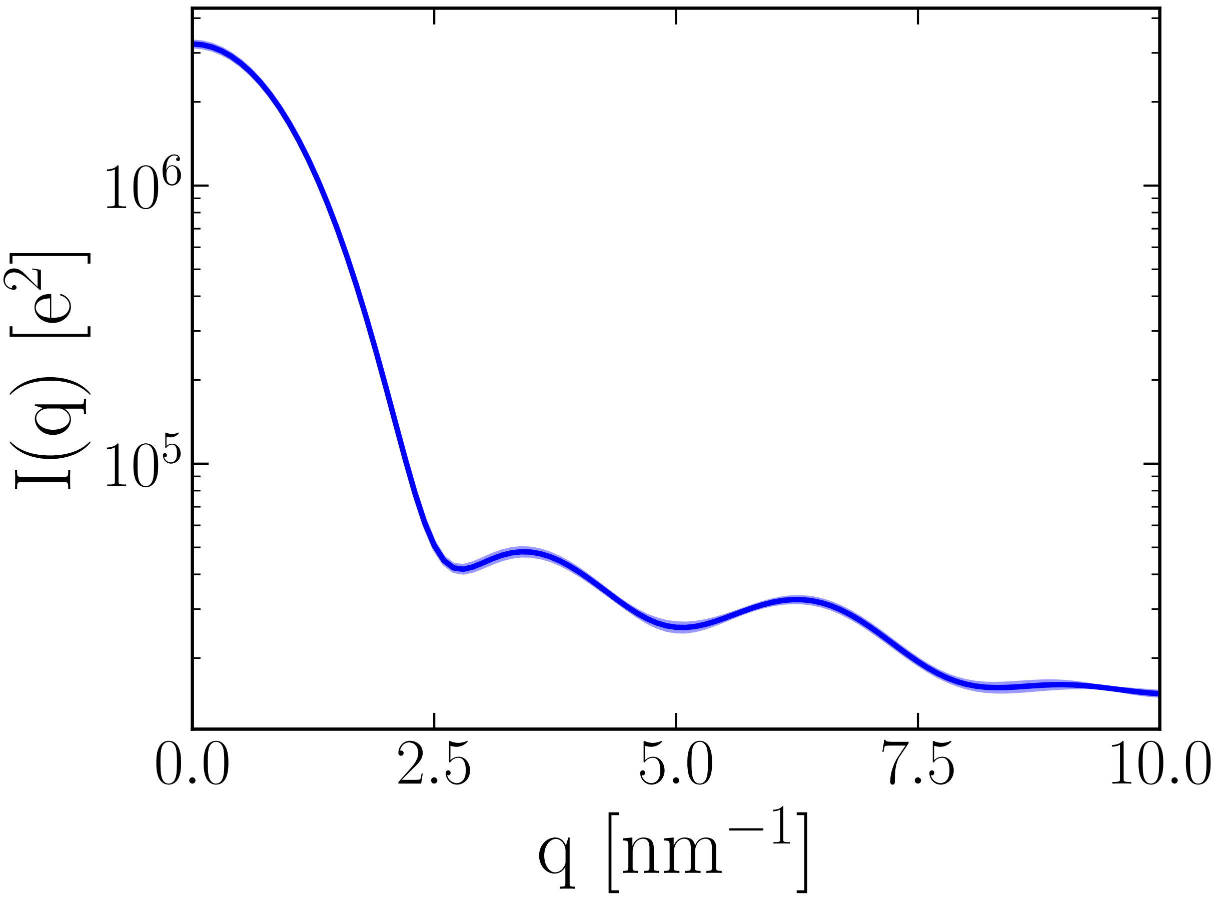


Figure S1: Scattering profile for lysozyme (PDB code: 193L) computed using SWAXS-AMDE for the purpose of validation. The shaded regions around the scattering curve represent the error bars in the SWAXS-AMDE calculation. The SWAXS-AMDE predicted I(q) is in excellent quantitative agreement with the results reported by Chen and Hub[12]

## S.4 Selecting Representative Simulation Frames for Scattering Analysis.

A calculation of the explicit water scattering intensities [I(q)] using all the $10^5$ simulation frames in the trajectory would be prohibitively expensive. Previous explicit water scattering computations show that using around 500 simulation frames is sufficient to obtain converged estimates.[12,14] In this study, the scattering intensities and their error bars for each simulation system are obtained from the block averaging of 5000 simulation frames (five blocks of a 1000 simulation frames each). The 5000 successive simulation frames for analysis are chosen such that the mean and standard deviation in $R_g$ for the selected frames is closest to the mean and standard deviation in $R_g$ for all the $10^5$ frames collected during the simulation. The mean and standard deviation in $R_g$ of the selected frames are compared to the mean and standard deviation in $R_g$ of all the simulation frames in Tab. S1.

Table S1: Comparison of the mean and standard deviation (Std.) in the radius of gyration ($R_g$) of the polyampholyte from all the simulation frames to the mean and standard deviation (Std.) in the radius of gyration ($R_g$) of the polyampholyte for the 5000 frames selected for scattering analysis.

| Force Field Combination | Polyampholyte Sequence | Mean $R_g$ All [Å] | Std. in $R_g$ All [Å] | Mean $R_g$ Selected [Å] | Std. in $R_g$ Selected [Å] |
|---|---|---|---|---|---|
| FF19O | $(EK)_{16}$ | 15.47 | 2.17 | 15.44 | 2.24 |
| FF19O | $(E_2K_2)_8$ | 18.19 | 3.10 | 18.19 | 3.11 |
| FF19O | $(E_4K_4)_4$ | 14.96 | 0.27 | 14.96 | 0.26 |
| OFF99 | $(EK)_{16}$ | 17.41 | 2.93 | 17.31 | 3.04 |
| OFF99 | $(E_2K_2)_8$ | 19.00 | 3.38 | 19.02 | 3.29 |
| OFF99 | $(E_4K_4)_4$ | 16.33 | 2.79 | 16.28 | 2.72 |
| TFF99 | $(EK)_{16}$ | 12.82 | 1.67 | 12.81 | 1.64 |
| TFF99 | $(E_2K_2)_8$ | 11.39 | 0.32 | 11.39 | 0.33 |
| TFF99 | $(E_4K_4)_4$ | 12.37 | 1.80 | 12.37 | 1.80 |

## S.5 Quantifying the Errors from the Computed Scattering Profiles

The errors of the computed scattering profiles with respect to the experimental data are quantified using the $\chi^2$ metric which is represented in Eq. S.4.

$$\chi^2 = \frac{1}{N}\sum_{i=1}^{N}\left[\frac{fI_{comp}(q_i) - I_{exp}(q_i)}{\sigma_{exp}(q_i)}\right]^2 \tag{S.4}$$

The $\chi$ values for all nine simulations with respect to the experimental data are reported in Tab. S2. The $\chi$ value reduces as the simulation model is changed from TFF99 to OFF99, quantifying the specific improvements due to the use of the OPC water model [except for $(E_4K_4)_4$, for which both TFF99 and OFF99 perform similarly]. The $\chi$ value further reduces as the simulation model is changed from OFF99 to FF19O [except for $(E_2K_2)_8$, for which both FF19O and OFF99 perform similarly], quantifying the specific improvements due to the use of the AMBER ff19SB atomistic force fields for protein.

Table S2: $\chi$ values for the nine simulations (three force field combinations * three polyampholyte sequences) with respect to the experimental data for that polyampholyte sequence.

| Polyampholyte Sequence | Force Field Combination | $\chi$ |
|---|---|---|
| $(EK)_{16}$ | TFF99 | 4.76 |
| $(EK)_{16}$ | OFF99 | 3.77 |
| $(EK)_{16}$ | FF19O | 2.00 |
| $(E_2K_2)_8$ | TFF99 | 6.04 |
| $(E_2K_2)_8$ | OFF99 | 1.92 |
| $(E_2K_2)_8$ | FF19O | 2.06 |
| $(E_4K_4)_4$ | TFF99 | 5.29 |
| $(E_4K_4)_4$ | OFF99 | 5.96 |
| $(E_4K_4)_4$ | FF19O | 1.40 |

## S.6 Ramachandran Plots for the Polyampholytes during Equilibration

The Ramachandran plots for each sequence of the EK polyampholyte are calculated by sorting the $\phi - \psi$ distribution into $2.5^0$*$2.5^0$ bins. The 32 $\phi - \psi$ angles from the $10^5$ frames (3.2*$10^6$ $\phi - \psi$ angles in total) during the first 4 $\mu$s of the simulation (equilibration) are represented as Ramachandran plots in Fig. S2. The PMFs shown in Fig. S2 are calculated using -log(counts) in each bin. The Ramachandran plots for each polyampholyte sequence for the TFF99 combination (during equilibration) are shown in Fig. S2(A)-(C). The Ramachandran plots for each polyampholyte sequence for the OFF99 combination (during equilibration) are shown in Fig. S2(D)-(F). The Ramachandran plots for each polyampholyte sequence for the FF19O combination (during equilibration) are shown in Fig. S2(G)-(I). The dihedral angle space sampled by the simulations during equilibration (0-4 $\mu$s) is the same as the dihedral angle space sampled by the simulations during production (4-8 $\mu$s), which indicates convergence of the simulations. For a mathematical description of the alpha-helix and beta-sheet regions in the Ramachandra plot and for a visual grouping of the various amino acid folds, we refer the reader to supplementary figure 20 of Ref. 15.

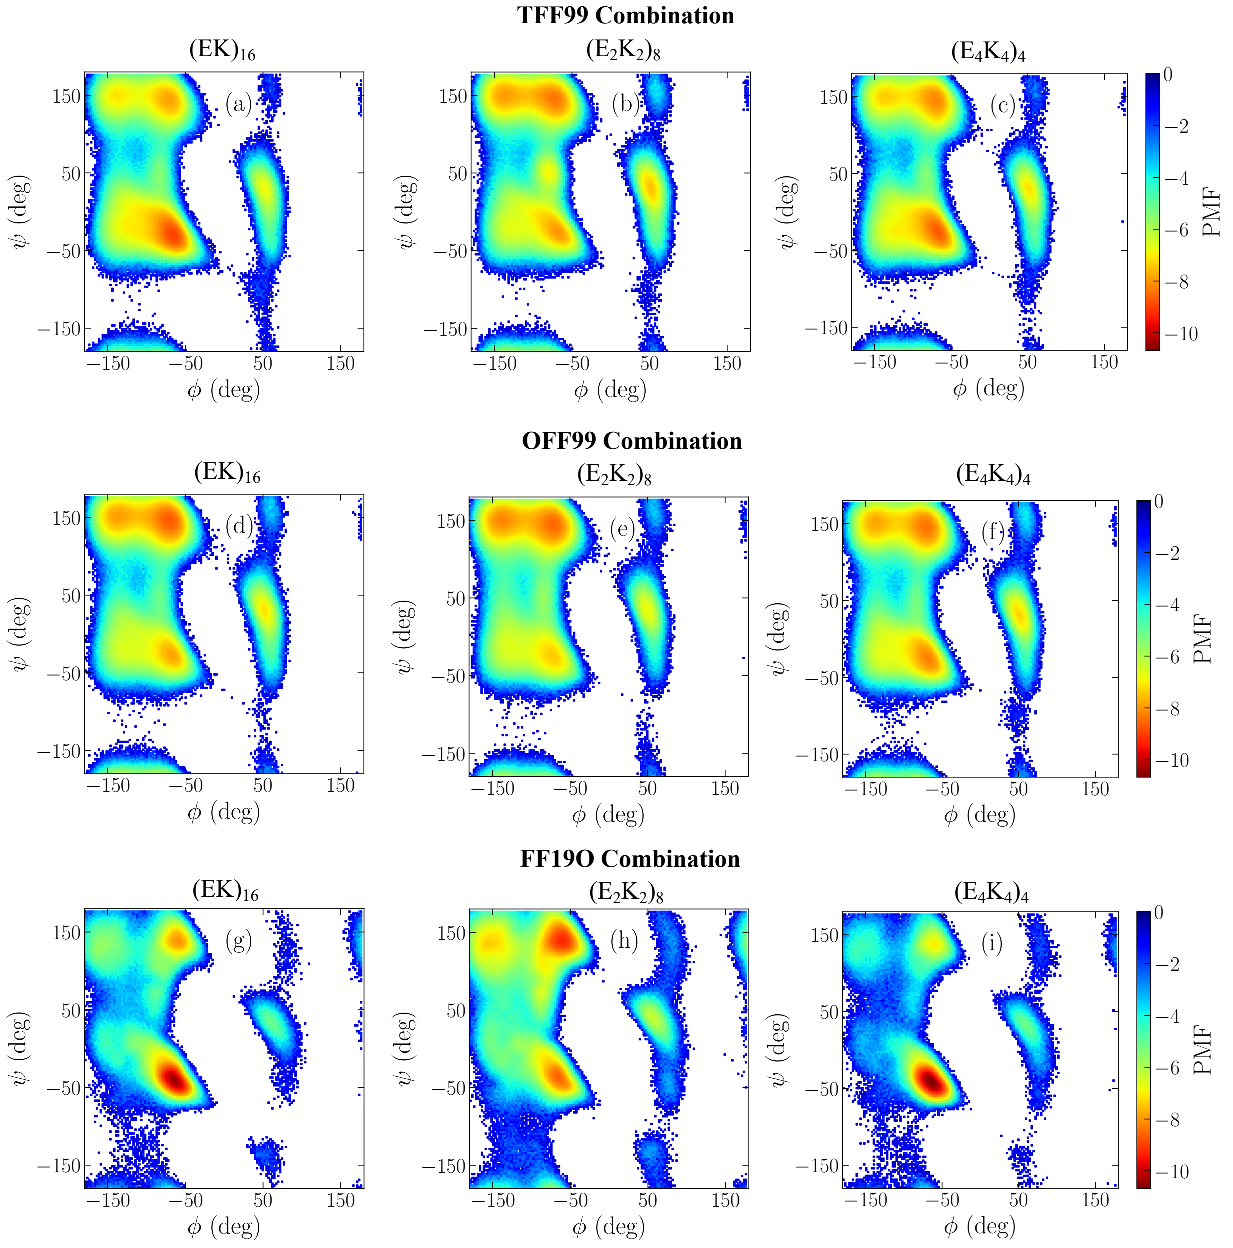


Figure S2: **Ramachandran plots for all nine simulations (three force field combinations * three polyampholyte sequences).** All of the Ramachandran plots are obtained from the first 4 $\mu$s of the simulation. The Ramachandran plots for the TFF99 combination are shown for the three polyampholyte sequences in (A)-(C) respectively. The Ramachandran plots for the OFF99 combination are shown for the three polyampholyte sequences in (D)-(F) respectively. The Ramachandran plots for the FF19O combination are shown for the three polyampholyte sequences in (G)-(I) respectively.

## S.7 Quantifying Errors by using a Constant Parameter to Account for Uncertainties in the Background Subtraction

The computed scattering profiles from the FF19O scattering profile compare well with respect to the experimental profiles up to a $q$ value of 0.3 Å$^{-1}$. One of the reasons for the discrepancy between the computed scattering profile and the experimental scattering profile at high-$q$ ($q > 0.3$ Å$^{-1}$) could be the uncertainties in the experimental background subtraction procedure. To account for this discrepancy, a constant parameter ($c$) is added to the computed scattering profile during error minimization, which is represented in Eq. S.5. Adding a constant parameter reduces the $\chi$ value for all three polyampholyte sequences as quantified in Tab. S3 (in comparison to the error minimization using Eq. S.4). The improved fit by adding the constant parameter ($c$) is also apparent visually from Fig. S3.

$$\chi^2 = \frac{1}{N} \sum_{i=1}^{N} \left[ \frac{\left(fI_{comp}(q_i) + c\right) - I_{exp}(q_i)}{\sigma_{exp}(q_i)} \right]^2 \tag{S.5}$$

Table S3: $\chi$ values from the two methods of error minimization for the FF19O force field combination. The FF19O scattering profiles are compared to the experiments first by only scaling the computed profiles and second by scaling the computed profiles and adding a constant parameter to account for the uncertainties in the background subtraction.

| Polyampholyte Sequence | Use of Constant Parameter during Minimization | $\chi$ |
|---|---|---|
| $(EK)_{16}$ | No | 2.00 |
| $(EK)_{16}$ | Yes | 1.74 |
| $(E_2K_2)_8$ | No | 2.06 |
| $(E_2K_2)_8$ | Yes | 1.93 |
| $(E_4K_4)_4$ | No | 1.40 |
| $(E_4K_4)_4$ | Yes | 0.82 |

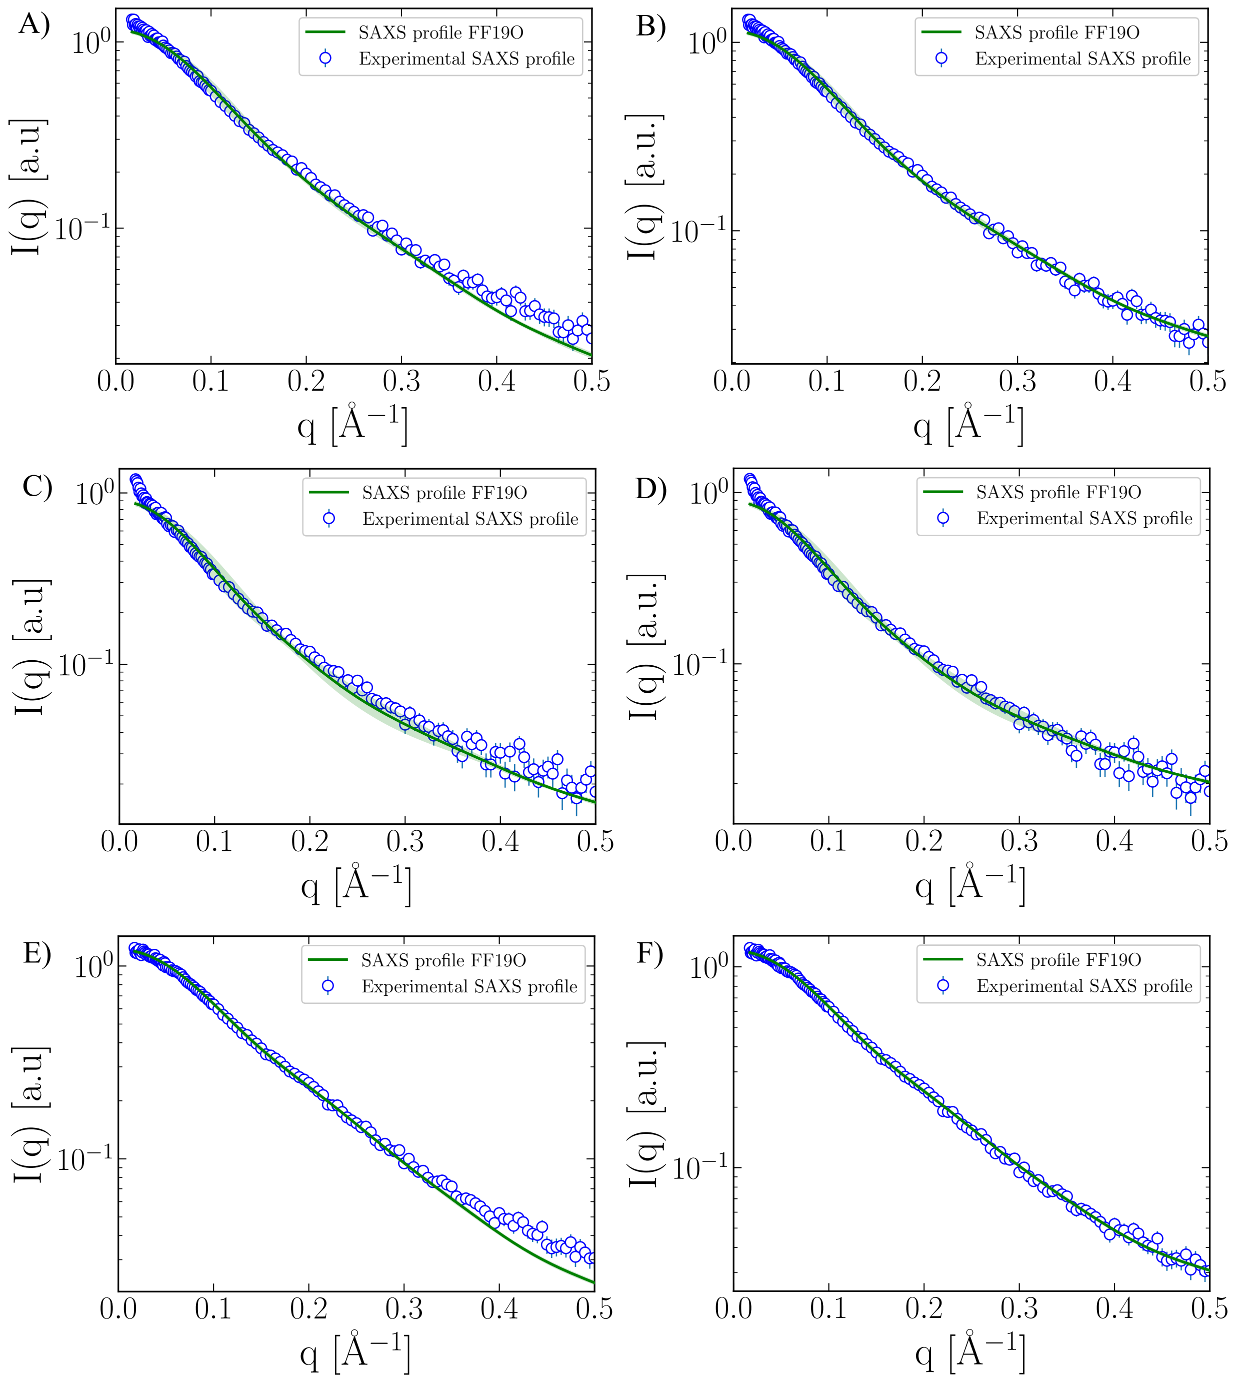


Figure S3: **Comparison of computed scattering profiles for the FF19O combination to the experimental data**. (A), (C), and (E) do not include a constant parameter to account for uncertainties in background subtraction. (B), (D), and (F) include a constant parameter to account for uncertainties in background subtraction. Comparison of the scattering profiles for the $(EK)_{16}$ polyampholyte without and with the constant parameter are shown in (A)-(B) respectively. Comparison of the scattering profiles for the $(E_2K_2)_8$ polyampholyte without and with the constant parameter are shown in (C)-(D) respectively. Comparison of the scattering profiles for the $(E_4K_4)_4$ polyampholyte without and with the constant parameter are shown in (E)-(F) respectively.

# References


(1) Tien, M. Z.; Sydykova, D. K.; Meyer, A. G.; Wilke, C. O. PeptideBuilder: A simple Python library to generate model peptides. *PeerJ* **2013**, *1*, e80.

(2) Onufriev, A.; Bashford, D.; Case, D. A. Modification of the generalized Born model suitable for macromolecules. *J. Phys. Chem. B* **2000**, *104*, 3712–3720.

(3) Phillips, J. C.; Hardy, D. J.; Maia, J. D.; Stone, J. E.; Ribeiro, J. V.; Bernardi, R. C.; Buch, R.; Fiorin, G.; Hénin, J.; Jiang, W., et al. Scalable molecular dynamics on CPU and GPU architectures with NAMD. *J. Chem. Phys.* **2020**, *153*.

(4) Case, D. A.; Aktulga, H. M.; Belfon, K.; Cerutti, D. S.; Cisneros, G. A.; Cruzeiro, V. W. D.; Forouzesh, N.; Giese, T. J.; Götz, A. W.; Gohlke, H., et al. AmberTools. *J. Chem. Inf. Model.* **2023**, *63*, 6183–6191.

(5) Hopkins, C. W.; Le Grand, S.; Walker, R. C.; Roitberg, A. E. Long-time-step molecular dynamics through hydrogen mass repartitioning. *J. Chem. Theory Comput.* **2015**, *11*, 1864–1874.

(6) Martínez, L.; Andrade, R.; Birgin, E. G.; Martínez, J. M. PACKMOL: A package for building initial configurations for molecular dynamics simulations. *J. Comput. Chem.* **2009**, *30*, 2157–2164.

(7) Case, D. A.; Aktulga, H. M.; Belfon, K.; Ben-Shalom, I.; Brozell, S. R.; Cerutti, D. S.; Cheatham III, T. E.; Cruzeiro, V. W. D.; Darden, T. A.; Duke, R. E., et al. *Amber 2021*; University of California, San Francisco, 2021.

(8) Park, S.; Bardhan, J. P.; Roux, B.; Makowski, L. Simulated x-ray scattering of protein solutions using explicit-solvent models. *J. Chem. Phys.* **2009**, *130*.

(9) Ponti, A. Simulation of magnetic resonance static powder lineshapes: a quantitative assessment of spherical codes. *J. Magn. Reson.* **1999**, *138*, 288–297.

(10) Prince, E. *International Tables for Crystallography, Volume C: Mathematical, physical and chemical tables*; Springer Science & Business Media, 2004.

(11) Sorenson, J. M.; Hura, G.; Glaeser, R. M.; Head-Gordon, T. What can x-ray scattering tell us about the radial distribution functions of water? *J. Chem. Phys.* **2000**, *113*, 9149–9161.

(12) Chen, P.-c.; Hub, J. S. Validating solution ensembles from molecular dynamics simulation by wide-angle X-ray scattering data. *Biophys. J.* **2014**, *107*, 435–447.

(13) Abraham, M. J.; Murtola, T.; Schulz, R.; Páll, S.; Smith, J. C.; Hess, B.; Lindahl, E. GROMACS: High performance molecular simulations through multi-level parallelism from laptops to supercomputers. *SoftwareX* **2015**, *1*, 19–25.

(14) Knight, C. J.; Hub, J. S. WAXSiS: a web server for the calculation of SAXS/WAXS curves based on explicit-solvent molecular dynamics. *Nucleic Acids Res.* **2015**, *43*, W225–W230.

(15) Huang, J.; Rauscher, S.; Nawrocki, G.; Ran, T.; Feig, M.; De Groot, B. L.; Grubmüller, H.; MacKerell Jr, A. D. CHARMM36m: an improved force field for folded and intrinsically disordered proteins. *Nat. Methods* **2017**, *14*, 71–73.
